# Supplementary material for: Computing the Haar state on ${\mathbb{O}(SL_q(3))}$
Source: arXiv:2301.12683 source file (2024-04-22)
Supplement: Supplementary file 1 [file appendix_A.tex]

\section{Source Matrix and its Solution} \label{apd:a}

\noindent The solution to the source matrix is 
\begin{equation*}
    \begin{split}
        h(aek(ceg)^{m-1})&=\frac{(-q)^{3m-2}(q^2-1)^3(q^4-1)(1+q^4-q^2-q^{2m+2})}{q(q^{2m}-1)^2(q^{2m+2}-1)^2(q^{2m+4}-1)}\\
        h(afh(ceg)^{m-1})&=\frac{(-q)^{3m-2}(q^2-1)^4(q^4-1)}{(q^{2m}-1)^2(q^{2m+2}-1)^2(q^{2m+4}-1)}\\
        h(bdk(ceg)^{m-1})&=\frac{(-q)^{3m-2}(q^2-1)^4(q^4-1)}{(q^{2m}-1)^2(q^{2m+2}-1)^2(q^{2m+4}-1)}\\
        h(bfgcdh(ceg)^{m-2})&=\frac{(-q)^{3m-2}(q^2-1)^4(q^4-1)}{(q^{2m}-1)^2(q^{2m+2}-1)^2(q^{2m+4}-1)}\\
        h(bfg(ceg)^{m-1})&=\frac{(-q)^{3m-1}(q^2-1)^3(q^4-1)}{(q^{2m}-1)(q^{2m+2}-1)^2(q^{2m+4}-1)}\\
        h(cdh(ceg)^{m-1})&=\frac{(-q)^{3m-1}(q^2-1)^3(q^4-1)}{(q^{2m}-1)(q^{2m+2}-1)^2(q^{2m+4}-1)}\\
        h((ceg)^{m})&=\frac{(-q)^{3m}(q^2-1)^2(q^4-1)}{(q^{2m+2}-1)^2(q^{2m+4}-1)}.
    \end{split}
\end{equation*}
For the entries of the source matrix of order $m$, see Table~\ref{tab:source} on the next page.

\begin{landscape}
%\begin{TAB}(r,0cm,0cm)[3pt]
\begin{table}[htb!]
    \centering
    \caption{The source matrix with all its entries.}
\resizebox{1.65\textheight}{!}{
\begin{tabular}{c|cccccccc}
%{c|ccccccc}
%\hline
 & $aekceg$ & $afhceg$ & $bdkceg$ & $bfgcdh$ & $bfgceg$ & $cdhceg$ & $cegceg$ & LHS \\ \hline
$D_q$ & $1$ & $-q$ & $-q$ & $0$ & $q^2$ & $q^2$ & $-q^3$ & $h((ceg)^{m-1})$ \\
 $aekceg$&$\frac{q^2(q^{2n}-1)^2}{q^{2n}(q^2-1)^2}$  & $\frac{-q(q^{2n}-1)^2}{q^{2n}(q^2-1)}$ & $\frac{q^3(1-q^{2n})^3}{q^{4n}(q^2-1)^2}$ & $\frac{(q^3-q^{2n+1})(q^{2n}-1)^3}{q^{4n}(q^2-1)^2}$ & $\frac{(q^{2n}-1)^2}{q^{2n}}$ & $\frac{n(q^{2n}-1)^2}{q^{2n}}$ & $\frac{(q^{2n}-1)((n+1)q^4-2nq^2+n)}{q^{2n+1}(q^2-1)}$ & 0 \\
 $aekbfg$& 0 & $\frac{q^2(q^{2n}-1)^3}{q^{2n}(q^2-1)^3}$ & 0 & 0 & $\frac{-q(q^{2n}-1)^2}{q^{2n}(q^2-1)}$ & $\frac{-nq(q^{2n}-1)^2}{q^{2n}(q^2-1)}$ & $\frac{(q^{2n}-1)(n-(n+1)q^2)}{q^{2n}(q^2-1)}$ & 0 \\ 
 $aekcdh$& 0 & 0 & $\frac{q^4(q^{2n}-1)^3}{q^{4n}(q^2-1)^3}$ & $\frac{(q^{2n}-1)^3(q^{2n+2}-q^4)}{q^{4n}(q^2-1)^3}$ & $\frac{-q(q^{2n}-1)^2}{q^{2n}(q^2-1)}$ & $\frac{-nq(q^{2n}-1)^2}{q^{2n}(q^2-1)}$ & $\frac{(q^{2n}-1)(n-(n+1)q^2)}{q^{2n}(q^2-1)}$ & 0 \\
 $afhbdk$& 0 & 0 & 0 & $\frac{(q^{2n}-1)^3(q^{2n+2}-q^4)}{q^{4n}(q^2-1)^4}$ & $c_1$ & $c_2$ & $c_3$ & 0 \\
 $aekbdk$& 0 & 0 & 0 & 0 & $\frac{q^2(q^{2n}-1)^2}{q^{2n}(q^2-1)^2}$ & 0 & $\frac{q(q^{2n}-1)}{q^{2n}(q^2-1)}$ & 0 \\
 $aekafh$& 0 & 0 & 0 & 0 & 0 & $\frac{q^2(q^{2n}-1)^2}{q^{2n}(q^2-1)^2}$ & $\frac{q(q^{2n}-1)}{q^{2n}(q^2-1)}$ & 0 \\ %\hline
\end{tabular}
}
\label{tab:source}
\end{table}

%\end{TAB}
\begin{equation*}
    \begin{split}
        c_1&=\frac{(q^{2n}-1)^2(q^{2n-2}+(n-1)q^{2n}-(n-1)q^{2n+2}-1)}{q^{4n-3}(q^2-1)^3}\\
        c_2&=\frac{(q^{2n}-1)^2(nq^{2n-2}-(n-1)q^{2n}-1)}{q^{4n-3}(q^2-1)^3}\\
        c_3&=\frac{(q^{2n}-1)(q^{2n+4}-n(q^4-1)q^{2n}-q^2)}{q^{4n}(q^2-1)^2}
    \end{split}
\end{equation*}
\end{landscape}
