# Supplementary material for: Computing the Haar state on ${\mathbb{O}(SL_q(3))}$
Source: arXiv:2301.12683 source file (2024-04-22)
Supplement: Supplementary file 2 [file appendix_B.tex]

\section{Recursive Formula for Monomial $(cdh)^{m_1}(ceg)^{m_2}$}
\label{apd:b}

The explicit expression of (\ref{eq:3}) is:
\begin{equation*}
    \begin{split}
         &\frac{q^2(q^{m-i+1}-q^{-(m-i+1)})^2}{(1-q^2)^2}*h((cdh)^i(ceg)^{m-i})\\
         =&\frac{iq^{-2(m-i)-1}-(i-1)q^{2(m-i)+5}-q}{q^2-1}*h((cdh)^{i-1}(ceg)^{m-i+1})\\     
         &-\sum_{k=2}^{i-1}c_k*h((cdh)^{i-k}(ceg)^{m-i+k})-(1/q-q)^{i-2}q^{-2(m-i+1)}h((ceg)^{m})\\
    \end{split}
\end{equation*}
where:
\begin{equation*}
\begin{split}
    c_k=(1/q-q)^{k-2}{i\choose k}q^{-2(m-i+1)}+(q-1/q)^{k-2}q^{2k}{i-1\choose k}q^{2(m-i+1)}.
\end{split}
\end{equation*}
